# Supplementary material for: Domain-oriented Language Pre-training with Adaptive Hybrid Masking and Optimal Transport Alignment
Source: arXiv:2112.03024 source file (2021-12-01)
Supplement: Supplementary file 1 [file appendix.tex]

\clearpage
\section*{Appendix}
\appendix

\section{\tb{Cross Attention for \np}}
% As illustrated in Figure \ref{np},
% we first sample associated entitys from the entity association graph and put their content embeddings into a pair (shown in the middle of the figure).
Figure \ref{np} shows an illustration of the cross attention based approach for CEA.
First, given two entities (associated with each other), we obtain their content embeddings via Transformer.
Then the cross attention layer is used to learn a correlation matrix, indicating word-level correlations between two entities.
Specifically, we multiply the correlation matrix with the central entity's content embeddings to generate a set of reconstructed content embeddings for the neighbor entity.
They are optimized to resemble the real content embeddings via the content reconstructing loss.
The loss enforces the cross attention layer to attend on highly correlated words and phrases for predicting the neighbors, while reducing the noise of unrelated contents.
Considering the central entity can also be viewed as a neighbor to the reconstructed entity, we perform the reconstructing task in both directions.
The learned cross attention matrix is considered as the alignments.

\begin{figure}[h]
%\vspace{-0.3cm}
% \setlength{\textfloatsep}{0.3cm}
\setlength{\belowcaptionskip}{-6pt}
\centering
\includegraphics[width=0.46\textwidth]{./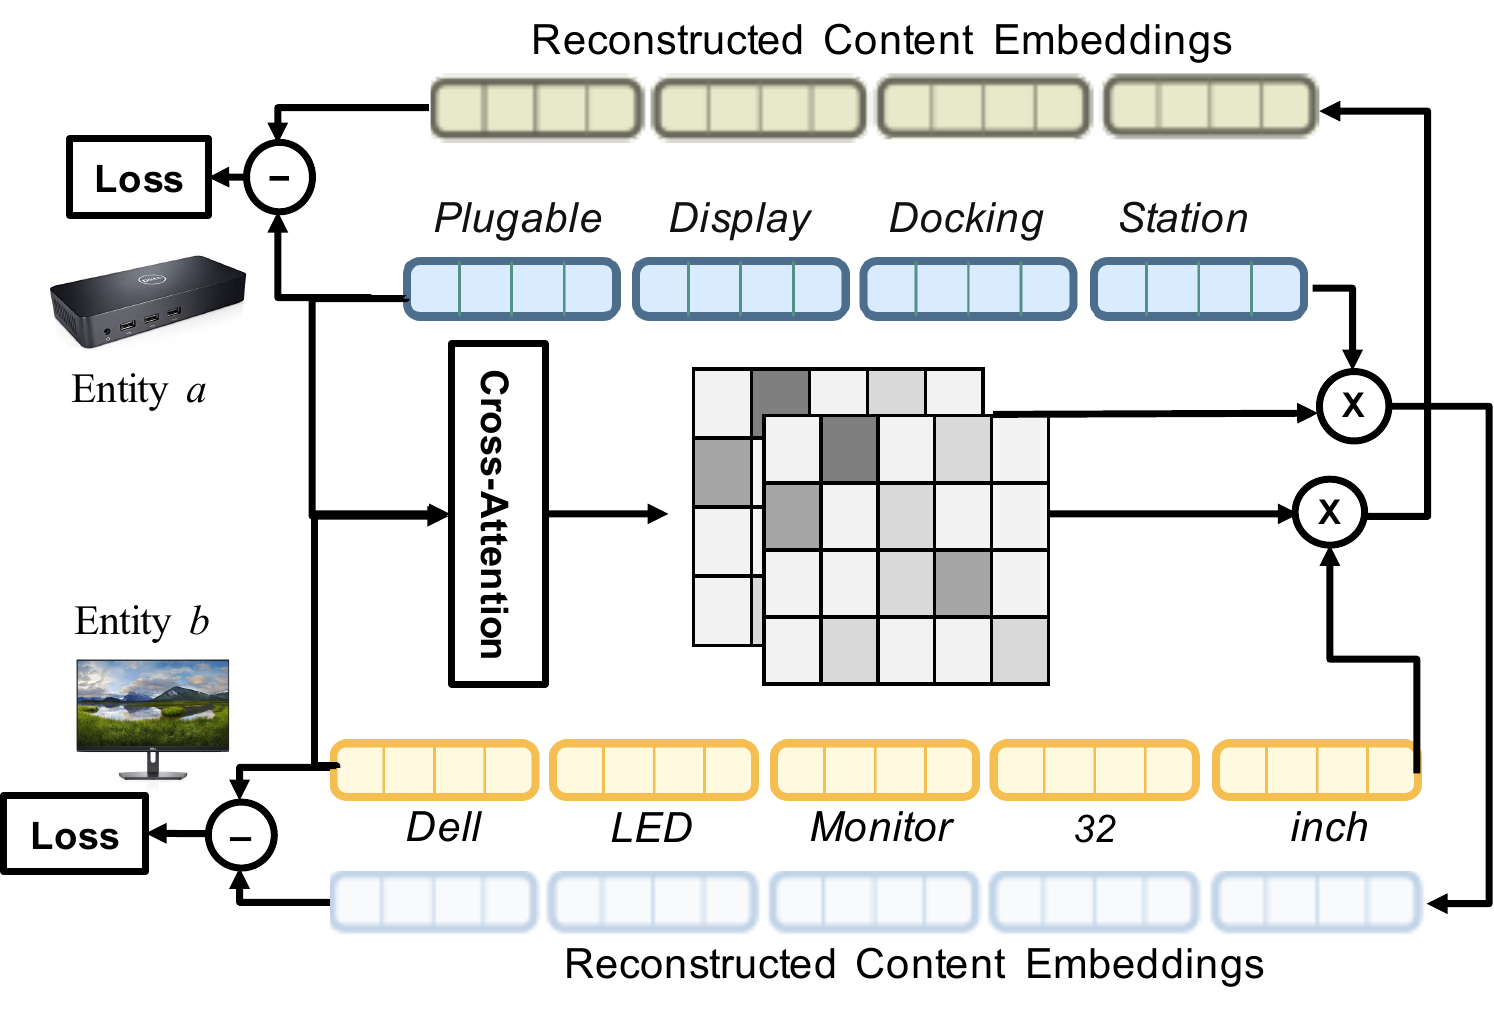}
% \vspace{-0.2cm}
\caption{Illustration of the cross attention approach for \np.}
\label{np}
% \vspace{-0.2cm}
\end{figure}

% \subsubsection{\tb{Content Embeddings}}
\noindent{\tb{Content Embeddings.}}
Given the entity pair $(a,b)$, we feed their contents into the language model (Transformer) respectively to get the contextual embeddings, denoted by $\{\bs{a_i}\}_{i=1}^n$ and $\{\bs{b_i}\}_{i=1}^m$.

% \subsubsection{\tb{Cross Attention Layer}}
\noindent{\tb{Cross Attention Layer.}}
We adopt the cross attention layer to generate two correlation matrices, i.e.,
\begin{equation}
\begin{aligned}
% \alpha_{ij} = \frac{\exp{(\bs{w_i}\bs{o_j})}}{\sum_{j'} \exp{(\bs{w_i}\bs{o_{j'}})}}, \;
% \beta_{ji} = \frac{\exp{(\bs{w_i}\bs{o_j})}}{\sum_{i'} \exp{(\bs{w_{i'}}\bs{o_{j}})}} ,
\alpha_{ij} = \frac{\exp{(\bs{a_i}\bs{b_j})}}{\sum_{j'} \exp{(\bs{a_i}\bs{b_{j'}})}}, \;
\beta_{ji} = \frac{\exp{(\bs{a_i}\bs{b_j})}}{\sum_{i'} \exp{(\bs{a_{i'}}\bs{b_{j}})}} ,
\end{aligned}
\end{equation}
where $a_i$ indicates the $i^{th}$ word in the entity $a$'s content and $b_j$ represents the $j^{th}$ word in $b$. 
% The cross attention weight $\alpha_{ij}$ and $\beta_{ji}$ indicates the correlation between $w_i$ and $o_j$ in different directions.
The cross attention weight $\alpha_{ij}$ and $\beta_{ji}$ both indicates the correlation between $a_i$ and $b_j$, but using different normalizers.

\noindent{\tb{Reconstructed Embeddings.}}
% Using the attention weights, we compute a weighted average of the real content embeddings to generate a set of reconstructed embedding, i.e.,
Using the attention weights, we compute a weighted average of the real content embeddings, i.e.,
\begin{equation} \label{eq:aligned_features}
\begin{aligned}
\bs{a}'_i = \sum_{j} \alpha_{ij} \bs{b}_j \;,\; 
\bs{b}'_j = \sum_{i} \beta_{ji}  \bs{a}_i .
\end{aligned}
\end{equation}
where $\bs{a}'_i$ and $\bs{b}'_j$ are the reconstructed embeddings, they will be optimized to resemble the original content embeddings $\bs{a}_i$ and $\bs{b}_j$. 
% The negative effect of noise is minimized by the cross attention as it automatically assigns smaller weights to irrelevant contents.
% \subsubsection{\tb{Reconstructing Loss}}

\noindent{\tb{Reconstructing Loss.}}
We define the content reconstructing loss of a entity pair as the Euclidean distance between their real content embeddings to the reconstructed embeddings, i.e.,
\begin{equation}
    \begin{aligned}
        \langle a,b \rangle &= \sum_{i} ||\bs{a}_i-\bs{a}'_i||_2^2 + \sum_{j} ||\bs{b}_j-\bs{b}'_j||_2^2 \\
    \end{aligned}
\end{equation}
We use a triplet loss as the final loss to pull relevant entity pairs close while pushing irrelevant ones apart:
\begin{equation} 
    \begin{aligned}
        \mathcal{L}_{\text{\snp-A}} &= \max (0, 1+\langle a,b \rangle-\langle a,b^- \rangle), 
    \end{aligned}
\end{equation}
where $b^-$ is a randomly sampled negative entity that has no association with $a$. 

\section{Inexact Proximal point method for Optimal Transport}
Algorithm \ref{alg:ipot} describes the implementation for the IPOT algorithm \cite{chen2019improving,xie2020fast}, which is used in our Optimal Transport based alignment learning method to solve $\tb{T}^*$ efficiently.
For the proximity metric term $\mathcal{B}(\Tmat,\Tmat^{(t)})$ in Eq. (11), we eomply the generalized KL Bregman divergence
$\mathcal{B}(\Tmat, \Tmat^{(t)})=\sum_{i,j} \Tmat_{ij}\log \frac{\Tmat_{ij}}{\Tmat^{(t)}_{ij}}-\sum_{i,j} \Tmat_{ij} + \sum_{i,j} \Tmat^{(t)}_{ij}$ as the proximity metric. 
 Below $K$ is set to $1$ in practice, and $\odot$ is Hadamard product. 

\begin{algorithm}[H]
% \footnotesize
\caption{IPOT algorithm}
\label{alg:ipot}
\begin{algorithmic}[1]
\REQUIRE {Feature vectors 
 $\Xmat=\{\xv_i\}_1^n$, $\Ymat=\{\yv_j\}_1^m$  and generalized stepsize $1/\beta$, 
}
\ENSURE $\Tmat$, $\langle \Tmat, \Cmat \rangle$

\STATE $\boldsymbol{\sigma}=\frac{1}{m}\mathbf{1_m}$, $\Tmat^{(1)} = \mathbf{1_n} \mathbf{1_m}^\top$
\STATE $\Cmat_{ij} = c(\xv_i, \yv_j)$, $\Amat_{ij} = {\rm e}^{-\frac{\Cmat_{ij}}{\beta}}$
\FOR{$t=1,2,3\ldots$}
    \STATE $\Qmat = \Amat \odot \Tmat^{(t)}$  {// $\odot$ is Hadamard product}
    %\quad \quad \quad // $\odot$ is Hadamard product
    \FOR{$k=1,\ldots K$} 
        \STATE $\boldsymbol{\delta} = \frac{1}{n\Qmat{\boldsymbol{\sigma}}}$, $\boldsymbol{\sigma} = \frac{1}{m\Qmat^\top\boldsymbol{\delta}}$
    \ENDFOR
    \STATE $\Tmat^{(t+1)} = \text{diag}(\boldsymbol{\delta})\Qmat\text{diag}(\boldsymbol{\sigma})$
\ENDFOR
% \STATE $\Lcal_{\text{ot}} = \langle \Tmat, \Cmat \rangle$
\STATE \textbf{Return} $\Tmat$, $\langle \Tmat, \Cmat \rangle$
\end{algorithmic}
\end{algorithm}
